# Supplementary material for: Enhanced nematic fluctuations near an antiferromagnetic Mott insulator and possible application to high-$T_{c}$ cuprates
Source: arXiv:1703.02210 source file (2019-04-23)
Supplement: Supplementary file 1 [file SupplementalMaterial.pdf]

# Supplemental Material for "Enhanced nematic fluctuations near the Mott insulating phase of high-$T_c$ cuprates"

Peter P. Orth,[1] Bhilahari Jeevanesan,[2] Rafael M. Fernandes,[3] and Jörg Schmalian[2,4]

[1]Department of Physics and Astronomy, Iowa State University, Ames, Iowa 50011, USA
[2]Institute for Theory of Condensed Matter, Karlsruhe Institute of Technology (KIT), 76131 Karlsruhe, Germany
[3]School of Physics and Astronomy, University of Minnesota, Minneapolis, Minnesota 55455, USA
[4]Institute for Solid State Physics, Karlsruhe Institute of Technology (KIT), 76131 Karlsruhe, Germany

(Dated: March 5, 2017)

## CONTENTS

S1. Derivation of $t-J-K$ model Hamiltonian from three-band Hubbard model 8
S1.A. Strong-coupling expansion 9
S1.B. Derivation of biquadratic spin exchange $K_0$ from microscopic Hamiltonian 9
S1.C. Analysis of bare biquadratic exchange coupling constant $K_0$ 11
S1.D. Renormalization of biquadratic exchange coupling $K$ by quadrupolar oxygen density fluctuations 13

S2. Nematic susceptibility within a soft-spin description of the half-filled $t-J-K$-model 13
S2.A. Nematic susceptibility $\chi_{\text{nem},0}(r,T)$ 14
S2.B. Large-$N$ analysis of the nematic susceptibility 16

S3. Spin-wave treatment of $t-J-K$ model at half-filling 17

S4. Details on the Monte-Carlo simulations 18

References 18

## S1. Derivation of $t-J-K$ model Hamiltonian from three-band Hubbard model

The starting point of a microscopic derivation of the biquadratic spin exchange term in the $t-J-K$ model in Eq. (1) of the main text is the three-band Hubbard model [1]: $H = H_0 + H_U + H_V$ with parts

$$H_0 = \sum_{\boldsymbol{R}_i,\sigma}\Big\{(\epsilon_p-\epsilon_d)n^p_{i\sigma} + t_{pd}\sum_u\Big[(-1)^u d^\dagger_{i\sigma}p_{i+u\sigma} + \text{h.c}\Big] + t_{pp}\sum_{u'}\Big[(-1)^{u'}p^\dagger_{i+\frac{\hat{x}}{2}\sigma}p_{i+\frac{\hat{x}}{2}+u'\sigma} + \text{h.c.}\Big]\Big\} \tag{S.1}$$

$$H_U = \sum_{\boldsymbol{R}_i}\Big(U_{dd}n^d_{i\uparrow}n^d_{i\downarrow} + U_{pp}\sum_{u=\frac{\hat{x}}{2},\frac{\hat{y}}{2}} n^p_{i+u\uparrow}n^p_{i+u\downarrow}\Big) \tag{S.2}$$

$$H_V = \sum_{\boldsymbol{R}_i}\Big(V_{pd}\sum_u n^d_i n^p_{i+u} + V_{pp}\sum_{u'} n^p_{i+\frac{\hat{x}}{2}}n^p_{i+\frac{\hat{x}}{2}+u'}\Big)\,. \tag{S.3}$$

Here, $d^\dagger_{i\sigma}$ creates a Cu ($3d_{x^2-y^2}$) hole with spin $\sigma$ at Bravais lattice site $\boldsymbol{R}_i$. The operators $p^\dagger_{i+\frac{\hat{x}}{2}\sigma}$ and $p^\dagger_{i+\frac{\hat{y}}{2}\sigma}$ create O ($2p_x$) and ($2p_y$) holes in the same unit cell $\boldsymbol{R}_i$, respectively. The vacuum is defined as filled $Cu^+$ ($d^{10}$) and $O^{2-}$ ($p^6$) states. We define the total number of Cu holes with spin $\sigma$ in unit cell $\boldsymbol{R}_i$ as $n^d_{i\sigma} = d^\dagger_{i\sigma}d_{i\sigma}$ and the Cu hole density as $n^d_i = \sum_\sigma n^d_{i\sigma}$. The corresponding operators for oxygen holes read $n^p_{i\sigma} = \sum_{u=\frac{\hat{x}}{2},\frac{\hat{y}}{2}} p^\dagger_{i+u\sigma}p_{i+u\sigma}$ and $n^p_i = \sum_\sigma n^p_{i\sigma}$.

The on-site energies of $d(p)$ orbitals are denoted $\epsilon_d(\epsilon_p)$ with $\Delta = \epsilon_p - \epsilon_d > 0$. The phase factors in the hopping terms arise from the overlap of orbital wavefunctions (see Fig. 1(b) of the main text) and are given by $(-1)^u = +1$ for $u = -\frac{\hat{x}}{2}, \frac{\hat{y}}{2}$, $(-1)^u = -1$ for $u = \frac{\hat{x}}{2}, -\frac{\hat{y}}{2}$ and $(-1)^{u'} = +1$ for $u' = \pm\frac{1}{2}(\hat{x}+\hat{y})$, $(-1)^{u'} = -1$ for $u' = \pm\frac{1}{2}(\hat{x}-\hat{y})$. The (unrestricted) sum $\sum_u$ runs over the four vectors connecting a central Cu site to its four neighboring O sites $u \in \{\pm\frac{\hat{x}}{2}, \pm\frac{\hat{y}}{2}\}$, and the sum $\sum_{u'}$ runs over the four vectors connecting an O $p_x$ orbital to its four $p_y$ neighbors $u' \in \{\pm\frac{1}{2}(\hat{x}\pm\hat{y})\}$. We consider on-site interactions $U_{dd}$ and $U_{pp}$ on both Cu and O sites as well as nearest-neighbor interactions $V_{pd}$ between Cu and O and $V_{pp}$ between oxygens.

### S1.A. Strong-coupling expansion

The hierarchy of energy scales suggests a strong-coupling expansion in small $t_{pd} \ll U_{dd} - \Delta, \Delta$, which yields a description in terms of localized Cu spins coupled to mobile O holes. Note that in order to derive the biquadratic exchange interaction term $\propto K$ in Eq. (1) of the main text, one can focus on the case of singly occupied Cu sites, *i.e.*, all holes reside on the oxygen sites. In the strong coupling expansion we follow Ref. 2 (see also Ref. 3) that contains an expansion up to fourth order in $t_{pd}^4/[\Delta^n(U_{dd}-\Delta)^m]$ with $n+m=3$ within this subspace. At second order one finds a term that renormalizes $t_{pp}$ and a Cu-O Kondo like exchange coupling term

$$H_{dp}^{(2)} = 2t_{pd}^2\Big(\frac{1}{\Delta} + \frac{1}{U-\Delta}\Big) \sum_{i,u_1,u_2} (-1)^{u_1+u_2} \boldsymbol{s}_{i+u_1,i+u_2} \cdot \boldsymbol{S}_i \tag{S.4}$$

with (non-)local O spin operators $\boldsymbol{s}_{ij} = \frac{1}{2}\sum_{\tau,\tau'} p_{i\tau}^\dagger \boldsymbol{\sigma}_{\tau\tau'} p_{j\tau'}$ with $\boldsymbol{\sigma} = (\sigma^x, \sigma^y, \sigma^z)$ being a vector of Pauli matrices and Cu spin operators $\boldsymbol{S}_i = \frac{1}{2}\sum_{\tau,\tau'} d_{i\tau}^\dagger \boldsymbol{\sigma}_{\tau\tau'} d_{i\tau'}$. At fourth order, there appear further Cu-O Kondo-like exchange terms, the well-known Heisenberg Cu-Cu spin exchange term

$$H_J^{(4)} = J \sum_{\langle i,j\rangle} \boldsymbol{S}_i \cdot \boldsymbol{S}_j \tag{S.5}$$

with $J = t_{pd}^4\Big(\frac{2}{\Delta^3} + \frac{3}{2\Delta^2(U_{dd}-\Delta)} - \frac{1}{2\Delta(U_{dd}-\Delta)^2}\Big)$ and a term that renormalizes hopping and interactions among oxygen sites. Most importantly for our analysis, however, there also appears a Cu spin exchange term that depends on the hole occupation number of the intermediate O orbital

$$H_{J'} = -J' \sum_{i,\delta} n^p_{i+\frac{\delta}{2}} \boldsymbol{S}_i \cdot \boldsymbol{S}_{i+\delta} \tag{S.6}$$

with $J' = t_{pd}^4\Big(\frac{1}{\Delta^3} + \frac{1}{\Delta^2(U_{dd}-\Delta)} - \frac{1}{\Delta(U_{dd}-\Delta)^2} - \frac{1}{(U_{dd}-\Delta)^3}\Big)$ and $\delta = \{\pm\hat{x}, \pm\hat{y}\}$. After integration of oxygen density fluctuation, this term will give rise to the biquadratic spin exchange as we show below. Note that in the limit of large-$U_{dd}$, one finds $\lim_{U_{dd}\to\infty} J'/J = 1/2$, so this term is of the same order as the Heisenberg spin-exchange.

There also appear non-local manifestations of this term with $n_i^p$ being replaced by $n_{ij}^p = \sum_\sigma p_{i\sigma}^\dagger p_{j\sigma}$ and term that describes coupling of the (non-)local spin density on the intermediate oxygen site to the cross product of Cu spins $H_{ddp}^{(4)} \propto \big[-2i\sum_{\langle i,j\rangle,u_1,u_2} \boldsymbol{s}_{i+u_1,j+u_2} \cdot (\boldsymbol{S}_i \times \boldsymbol{S}_j)\big]$, which are, however, not the focus of our analysis.

### S1.B. Derivation of biquadratic spin exchange $K_0$ from microscopic Hamiltonian

To consider the effect of charge fluctuations on the oxygen sites, we rewrite the oxygen interaction part of the Hamiltonian $H_{U_{pp}} + H_{V_{pp}}$ in terms of total $n_i^p$ and relative oxygen density $\eta_i$ within unit cell $\boldsymbol{R}_i$:

$$n_i^p = n^p_{i+\frac{\hat{x}}{2}} + n^p_{i+\frac{\hat{y}}{2}} \tag{S.7}$$

$$\eta_i = n^p_{i+\frac{\hat{x}}{2}} - n^p_{i+\frac{\hat{y}}{2}}\,. \tag{S.8}$$

This allows to write the oxygen-density-dependent interaction between neighboring Cu spins in Eq. (S.6) as

$$H_{J'} = -\frac{J'}{2}\sum_i \Big[\eta_i\big(\boldsymbol{S}_i\cdot\boldsymbol{S}_{i+\hat{x}} - \boldsymbol{S}_i\cdot\boldsymbol{S}_{i+\hat{y}}\big) + \eta_{i-\hat{x}}\boldsymbol{S}_i\cdot\boldsymbol{S}_{i-\hat{x}} - \eta_{i-\hat{y}}\boldsymbol{S}_i\cdot\boldsymbol{S}_{i-\hat{y}} + n_i^p\big(\boldsymbol{S}_i\cdot\boldsymbol{S}_{i+\hat{x}} + \boldsymbol{S}_i\cdot\boldsymbol{S}_{i+\hat{y}}\big) + \sum_{\delta=\hat{x},\hat{y}} n^p_{i-\delta}\boldsymbol{S}_i\cdot\boldsymbol{S}_{i-\delta}\Big] \tag{S.9}$$

The on-site ($U_{pp}$) and nearest-neighbor ($V_{pp}, V_{pd}$) oxygen interaction terms in Eq. (S.2) and (S.3) take the form

$$H_{U_{pp}} + H_{V_{pp}} + H_{V_{pd}} = \frac{1}{N_L}\sum_{\boldsymbol{k}}\Big[U_{+,\boldsymbol{k}} n^p_{\boldsymbol{k}} n^p_{-\boldsymbol{k}} - U_{-,\boldsymbol{k}}\eta_{\boldsymbol{k}}\eta_{-\boldsymbol{k}} + \frac{V_{pp} f_{\boldsymbol{k}}}{4}(\eta_{\boldsymbol{k}} n^p_{-\boldsymbol{k}} - \eta_{-\boldsymbol{k}} n^p_{\boldsymbol{k}})\Big] + 2V_{pd} n_0^p \tag{S.10}$$

where we introduce the interactions $U_{\pm,\boldsymbol{k}} = \frac{V_{pp} f_{\boldsymbol{k}}}{4} \pm \frac{U_{pp}}{8}$ and we write the Fourier transform as $\eta_i = \frac{1}{N_L}\sum_{\boldsymbol{k}} \eta_{\boldsymbol{k}} e^{i\boldsymbol{k}\cdot\boldsymbol{R}_i}$ with total number of unit cells $N_L$. The lattice function is given by $f_{\boldsymbol{k}} = \sum_{\delta'} e^{-i\boldsymbol{k}\delta'} = 1 + e^{-ik_x} + e^{ik_y} + e^{i(k_y-k_x)}$.

Here, $\delta' \in \{0, \hat{x}, -\hat{y}, \hat{x}-\hat{y}\}$ denotes Bravais lattice vectors pointing to unit cells containing the four nearest-neighbor $p_y$ oxygen orbitals of a given oxygen $p_x$ orbital.

As required, Eq. (S.10) is invariant under the spatial symmetries of the system. In particular, it is invariant under fourfold $C_4$ rotation $C_4(x_i, y_i) = (-y_i, x_i)$, $C_4(k_x, k_y) = (-k_y, k_x)$. This follows from the transformation laws of the orbitals $p_{i+\frac{\hat{x}}{2}} \xrightarrow{C_4} p_{C_4(i)+\frac{\hat{y}}{2}}$ and $p_{i+\frac{\hat{y}}{2}} \xrightarrow{C_4} p_{C_4(i)-\frac{\hat{x}}{2}}$. The transformation laws for total and relative densities follow as $\eta_{\boldsymbol{k}} \xrightarrow{C_4} \frac{1}{2}(1-e^{-ik_x})n^p_{\boldsymbol{k}} - \frac{1}{2}(1+e^{-ik_x})\eta_{\boldsymbol{k}}$ and $n^p_{\boldsymbol{k}} \xrightarrow{C_4} \frac{1}{2}(1+e^{-ik_x})n^p_{\boldsymbol{k}} + \frac{1}{2}(e^{-ik_x}-1)\eta_{\boldsymbol{k}}$. Noting that $f_{\boldsymbol{k}} \xrightarrow{C_4} f_{C_4^{-1}(\boldsymbol{k})} = 1 + e^{-ik_y} + e^{-ik_x} + e^{-i(k_y+k_x)} = e^{-ik_y} f_{\boldsymbol{k}}$, one can easily show using $e^{i(k_x-k_y)} f_{\boldsymbol{k}} = f_{-\boldsymbol{k}}$ that Eq. (S.10) is invariant under $C_4$ rotations.

Since the operators $\eta_{\boldsymbol{k}}$ and $n^p_{\boldsymbol{k}}$ transform into each other under symmetry transformations (such as $C_4$), we need to treat them on equal footing when decoupling the interaction terms using a Hubbard-Stratonovich (HS) transformation. We introduce the vector $v_{\boldsymbol{k}} = (n^p_{\boldsymbol{k}}, \eta_{\boldsymbol{k}})^T$ and write $H_{U_{pp}} + H_{V_{pp}} = -\sum_{\boldsymbol{k}, k_x>0} v^\dagger_{\boldsymbol{k}} U^{-1}_{\boldsymbol{k}} v_{\boldsymbol{k}}$ with interaction matrix

$$U^{-1}_{\boldsymbol{k}} = \frac{2}{N_L}\begin{pmatrix} -\mathrm{Re}\, U_{+,\boldsymbol{k}} & i\frac{V_{pp}}{4}\mathrm{Im}\, f_{\boldsymbol{k}} \\ -i\frac{V_{pp}}{4}\mathrm{Im}\, f_{\boldsymbol{k}} & \mathrm{Re}\, U_{-,\boldsymbol{k}} \end{pmatrix} \longrightarrow U_{\boldsymbol{k}} = \frac{N_L}{2}\frac{1}{\left(\frac{V_{pp}}{4}\right)^2 |f_{\boldsymbol{k}}|^2 + \left(\frac{U_{pp}}{8}\right)^2}\begin{pmatrix} -\mathrm{Re}\, U_{-,\boldsymbol{k}} & i\frac{V_{pp}}{4}\mathrm{Im}\, f_{\boldsymbol{k}} \\ -i\frac{V_{pp}}{4}\mathrm{Im}\, f_{\boldsymbol{k}} & \mathrm{Re}\, U_{+,\boldsymbol{k}} \end{pmatrix}. \tag{S.11}$$

The HS transformation introduces the fields $\Phi_{\boldsymbol{k}} = (\psi_{\boldsymbol{k}}, \phi_{\boldsymbol{k}})$ and yields the action

$$S_{U_{pp}+V_{pp}} = \int_k (\Phi^\dagger_k U_k \Phi_k - \Phi^\dagger_k v_k - v^\dagger_k \Phi_k)\,, \tag{S.12}$$

where $k = (ik_n, \boldsymbol{k})$ combines Matsubara frequency $ik_n = 2\pi nT$ with temperature $T$ and momentum $\boldsymbol{k}$. We note that the fields $\Phi_k$ transform identical to $v_k$ in order that the action remains invariant under all symmetry transformations.

We have arrived at an action that is quadratic in oxygen hole operators. In a next step, we will perform the exact functional integration over these degrees of freedom. We focus on those terms in the action that are relevant for the derivation of the biquadratic exchange interaction $S = S_0 + S_{U_{pp}+V_{pp}} + S_{J'}$, which read explicitly

$$S = -\int_{q,k} \sum_{u,u'\sigma,\sigma'} p^\dagger_{qu\sigma} G^{-1}_{qu\sigma,ku'\sigma'} p_{ku'\sigma'} + \int_k \Phi^\dagger_k U_k \Phi_k\,, \tag{S.13}$$

where $u, u' \in \{x, y\}$ label $(p_x, p_y)$ orbitals and $\sigma, \sigma' \in \{\uparrow, \downarrow\}$ denote the spin direction. The inverse Green's function $G^{-1}(\boldsymbol{S}_i)$ in Eq. (S.13) contains the Cu spin operators $\boldsymbol{S}_i$ and is a sum of terms

$$G^{-1} = G^{-1}_0 + G^{-1}_{U_{pp}+V_{pp}} + G^{-1}_{J'} \tag{S.14}$$

Since all Green's functions are diagonal in spin space, $G^{-1} \propto \sigma^0$ with $\sigma^0 = \mathrm{diag}(1,1)$, we suppress the spin indices in the following and find

$$G^{-1}_{0;qu,qu'} = \big(iq_n - \Delta + \mu - 2V_{pd}\big)\tau^0 - t_{pp}\mathrm{Re}(h_{\boldsymbol{q}})\tau^x + t_{pp}\mathrm{Im}(h_{\boldsymbol{q}})\tau^y \tag{S.15}$$

$$G^{-1}_{U_{pp}+V_{pp};qu,ku'} + G^{-1}_{J';qu,ku'} = a_{0,q-k}\tau^0 + a_{z,q-k}\tau^z\,. \tag{S.16}$$

Here, $\tau^\alpha$ are Pauli matrices in orbital $(p_x, p_y)$ space, $\tau^0 = \mathrm{diag}(1,1)$ and we have defined the lattice function

$$h_{\boldsymbol{q}} = 1 - e^{iq_x} - e^{-iq_y} + e^{i(q_x-q_y)} \tag{S.17}$$

that describes oxygen hopping. We have also introduced the functions

$$a_{0,q-k} = \psi_{q-k} - \sum_{\boldsymbol{p}} \mathcal{S}_{\boldsymbol{p},\boldsymbol{q}-\boldsymbol{k}} h_m(\boldsymbol{p}, \boldsymbol{k}-\boldsymbol{q}) \tag{S.18}$$

$$a_{z,q-k} = \phi_{q-k} - \sum_{\boldsymbol{p}} \mathcal{S}_{\boldsymbol{p},\boldsymbol{q}-\boldsymbol{k}} h_\eta(\boldsymbol{p}, \boldsymbol{k}-\boldsymbol{q})\,. \tag{S.19}$$

These functions contain the HS fields $\psi_k$ and $\phi_k$ as well as the spin bilinear $\mathcal{S}_{\boldsymbol{p},\boldsymbol{q}} = \boldsymbol{S}_{\boldsymbol{p}} \cdot \boldsymbol{S}_{-\boldsymbol{p}-\boldsymbol{q}}$. Under a $C_4$ rotation it remains invariant $C_4(\mathcal{S}_{\boldsymbol{p},\boldsymbol{q}}) = \mathcal{S}_{\boldsymbol{p},\boldsymbol{q}}$. The interaction of Cu spins with the intermediate oxygen site [see Eq. (S.9)] is captured in Fourier space by the lattice functions

$$h_m(\boldsymbol{p}, \boldsymbol{k}) = \frac{J'}{2}\big(e^{ip_x} + e^{ip_y} + e^{-i(p_x+k_x)} + e^{-i(p_y+k_y)}\big) \tag{S.20}$$

$$h_\eta(\boldsymbol{p}, \boldsymbol{k}) = \frac{J'}{2}\big(e^{ip_x} - e^{ip_y} + e^{-i(p_x+k_x)} - e^{-i(p_y+k_y)}\big)\,. \tag{S.21}$$

Functional integration over $p^\dagger_{qu\sigma}$ and $p_{qu\sigma}$ yields the action

$$S = \int_k \Phi_k^\dagger U_k \Phi_k - \mathrm{Tr}\log(-G^{-1}) = \int_k \Phi_k^\dagger U_k \Phi_k + \frac{1}{2}\mathrm{Tr}[\{G_0(G^{-1}_{U_{pp}+V_{pp}} + G^{-1}_{J'})\}^2] + \dots \tag{S.22}$$

where the ellipsis stands for the zeroth, first and higher order terms. Focusing on the quadratic term, we write it as

$$S_2 = \frac{1}{2}\mathrm{Tr}[\{G_0(G^{-1}_{U_{pp}+V_{pp}} + G^{-1}_{J'})\}^2] = -\frac{1}{2}\int_q \sum_{\alpha,\beta\in\{0,z\}} a_{\alpha,q}a_{\beta,-q}\Pi^{\alpha\beta}_{-q}\,, \tag{S.23}$$

where we have introduced the response functions

$$\Pi^{\alpha\beta}_q = -\int_k \mathrm{Tr}\big[G_{0,k}(\tau^\alpha\sigma^0)G_{0,k+q}(\tau^\beta\sigma^0)\big]\,. \tag{S.24}$$

Performing the summation over Matsubara frequencies and setting the external frequency $iq_n$ to zero, they read

$$\Pi^{00}_{\boldsymbol{q}} = \int_{\boldsymbol{k}} \frac{2}{\epsilon^2_{\boldsymbol{k}+\boldsymbol{q}} - \epsilon^2_{\boldsymbol{k}}}\left\{\frac{\epsilon^2_{\boldsymbol{k}} + g_{+,\boldsymbol{k},\boldsymbol{q}}}{\epsilon_{\boldsymbol{k}}}\big[n_F(\tilde\Delta+\epsilon_{\boldsymbol{k}}) - n_F(\tilde\Delta-\epsilon_{\boldsymbol{k}})\big] - \frac{\epsilon^2_{\boldsymbol{k}+\boldsymbol{q}} + g_{+,\boldsymbol{k},\boldsymbol{q}}}{\epsilon_{\boldsymbol{k}+\boldsymbol{q}}}\big[n_F(\tilde\Delta+\epsilon_{\boldsymbol{k}+\boldsymbol{q}}) - n_F(\tilde\Delta-\epsilon_{\boldsymbol{k}+\boldsymbol{q}})\big]\right\} \tag{S.25}$$

$$\Pi^{z0}_{\boldsymbol{q}} = \int_{\boldsymbol{k}} \frac{2g_{-,\boldsymbol{k},\boldsymbol{q}}}{\epsilon^2_{\boldsymbol{k}+\boldsymbol{q}} - \epsilon^2_{\boldsymbol{k}}}\left\{\frac{n_F(\tilde\Delta+\epsilon_{\boldsymbol{k}}) - n_F(\tilde\Delta-\epsilon_{\boldsymbol{k}})}{\epsilon_{\boldsymbol{k}}} - \frac{n_F(\tilde\Delta-\epsilon_{\boldsymbol{k}+\boldsymbol{q}}) - n_F(\tilde\Delta-\epsilon_{\boldsymbol{k}+\boldsymbol{q}})}{\epsilon_{\boldsymbol{k}+\boldsymbol{q}}}\right\} \tag{S.26}$$

$$\Pi^{zz}_{\boldsymbol{q}} = \int_{\boldsymbol{k}} \frac{2}{\epsilon^2_{\boldsymbol{k}+\boldsymbol{q}} - \epsilon^2_{\boldsymbol{k}}}\left\{\frac{\epsilon^2_{\boldsymbol{k}} - g_{+,\boldsymbol{k},\boldsymbol{q}}}{\epsilon_{\boldsymbol{k}}}\big[n_F(\tilde\Delta+\epsilon_{\boldsymbol{k}}) - n_F(\tilde\Delta-\epsilon_{\boldsymbol{k}})\big] - \frac{\epsilon^2_{\boldsymbol{k}+\boldsymbol{q}} - g_{+,\boldsymbol{k},\boldsymbol{q}}}{\epsilon_{\boldsymbol{k}+\boldsymbol{q}}}\big[n_F(\tilde\Delta+\epsilon_{\boldsymbol{k}+\boldsymbol{q}}) - n_F(\tilde\Delta-\epsilon_{\boldsymbol{k}+\boldsymbol{q}})\big]\right\}, \tag{S.27}$$

and $\Pi^{0z}_{\boldsymbol{q}} = -\Pi^{z0}_{\boldsymbol{q}}$. Here, $n_F(x) = [\exp(x/T)+1]^{-1}$ is the Fermi function and we have defined $\tilde\Delta = \Delta - \mu$, $\epsilon_{\boldsymbol{q}} = t_{pp}|h_{\boldsymbol{q}}|$ and $g_{\pm,\boldsymbol{q},\boldsymbol{k}} = \frac{1}{2}t^2_{pp}\big(h^*_{\boldsymbol{q}}h_{\boldsymbol{q}+\boldsymbol{k}} \pm \text{c.c}\big)$. We note that the response functions $\Pi^{\alpha\beta}$ are only $C_2$ symmetric, but their sum as it appears in the action is always fully $C_4$ symmetric, which we have verified explicitly. Importantly, in the long wavelength limit, one finds that both $\lim_{|\boldsymbol{k}|\to 0}\Pi^{00} > 0$ and $\lim_{|\boldsymbol{k}|\to 0}\Pi^{zz} > 0$. This determines the sign of the biquadratic exchange coupling $K > 0$ as given in Eq. (1) of the main text.

Focusing on the bare biquadratic term arising from the product of the operators $\mathcal{S}_{\boldsymbol{p},\boldsymbol{q}}$ in Eq. (S.23), it is instructive to write it in real space as

$$S^{\mathcal{S}^2}_2 = -\frac{J'^2}{2}\sum_{i,j}\Big\{\Pi^{00}_{ji}\Big(\boldsymbol{S}_i\cdot\boldsymbol{S}_{i+\hat{x}} + \boldsymbol{S}_i\cdot\boldsymbol{S}_{i+\hat{y}}\Big)\Big(\boldsymbol{S}_j\cdot\boldsymbol{S}_{j+\hat{x}} + \boldsymbol{S}_j\cdot\boldsymbol{S}_{j+\hat{y}}\Big) \tag{S.28}$$
$$+ \Pi^{zz}_{ji}\Big(\boldsymbol{S}_i\cdot\boldsymbol{S}_{i+\hat{x}} - \boldsymbol{S}_i\cdot\boldsymbol{S}_{i+\hat{y}}\Big)\Big(\boldsymbol{S}_j\cdot\boldsymbol{S}_{j+\hat{x}} - \boldsymbol{S}_j\cdot\boldsymbol{S}_{j+\hat{y}}\Big) + 4\Pi^{z0}_{ji}\Big(\boldsymbol{S}_i\cdot\boldsymbol{S}_{i+\hat{x}}\Big)\Big(\boldsymbol{S}_j\cdot\boldsymbol{S}_{j+\hat{y}}\Big)\Big\}$$

with $\Pi_{ji} = \int_{\boldsymbol{q}} e^{-i\boldsymbol{q}\cdot(\boldsymbol{R}_j-\boldsymbol{R}_i)}\Pi_{-\boldsymbol{q}}$. The bare biquadratic exchange coupling $K_0$ follows as

$$K_0 = \frac{J'^2}{2}\Pi^{zz}_{ii} = \frac{J'^2}{2}\int_{\boldsymbol{q}}\Pi^{zz}_{\boldsymbol{q}}\,. \tag{S.29}$$

We note again that the action $S^{\mathcal{S}^2}_2$ is fully $C_4$ invariant and the interaction terms that involve spin operators in neighboring unit cells $i-\hat{x}$ and $i-\hat{y}$ arise from the the off-diagonal components $\Pi^{z0}_{ij}$. In Fig. S.1 we show the response functions $\Pi^{\alpha\beta}$ both in real and momentum space for a realistic choice of parameters $t_{pd} = 1$, $t_{pp} = 0.2$, $\Delta = 2.5$, $n_p = 0.05$, $U_{dd} = 9$, $U_{pp} = 3$, $V_{pp} = 2.0$, $V_{pd} = 1.0$ and temperature $T = 0.02$.

### S1.C. Analysis of bare biquadratic exchange coupling constant $K_0$

To gain some analytic understanding, we approximate the bare biquadratic coupling constant by

$$K_0 \approx \frac{J'^2}{2}\lim_{\boldsymbol{q}\to 0}\Pi^{zz}_{\boldsymbol{q}} = J'^2\int_{BZ}\frac{d^2q}{v_{BZ}}\frac{n_F(\xi_-) - n_F(\xi_+)}{\epsilon_{\boldsymbol{q}}}\,. \tag{S.30}$$

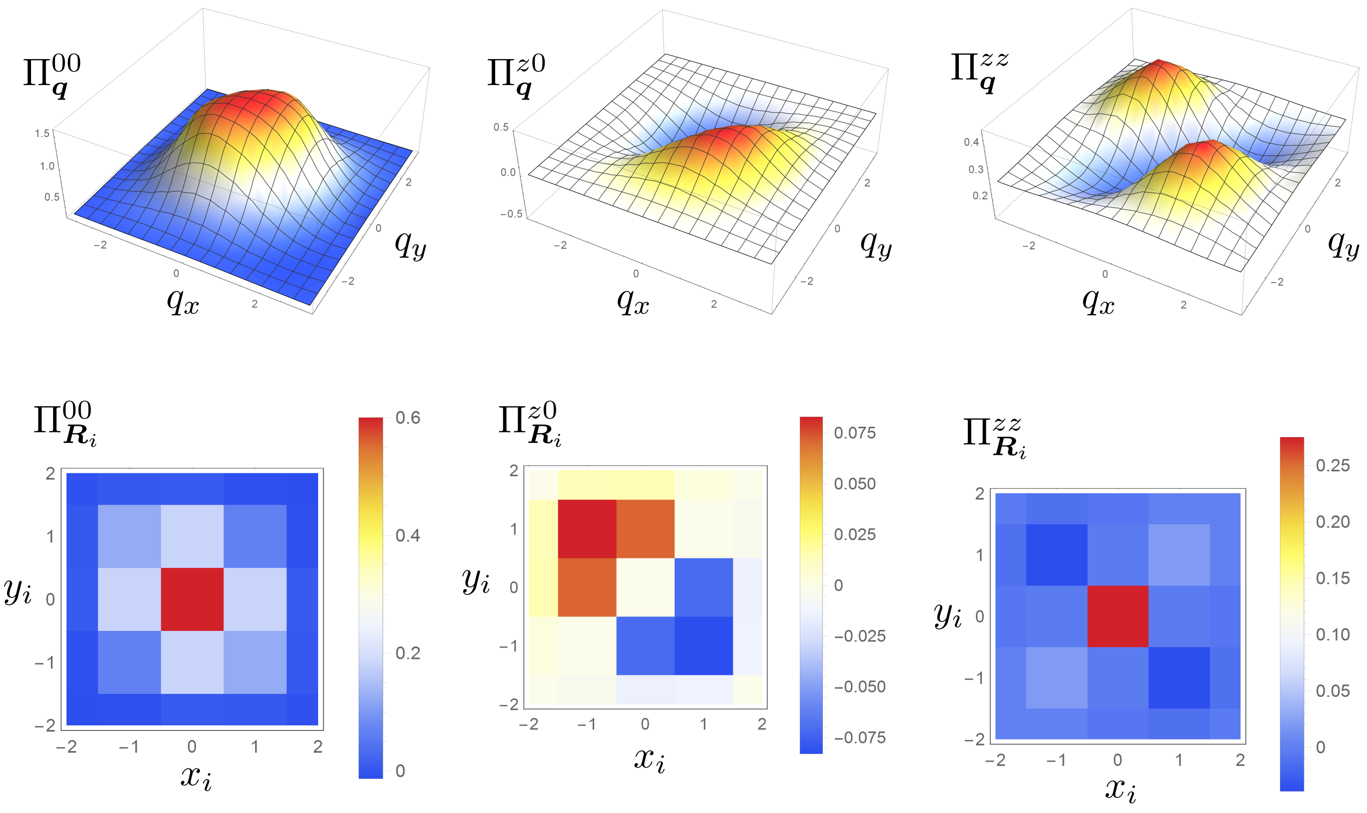


FIG. S.1. Response functions in momentum $\Pi^{\alpha\beta}_{\boldsymbol{q}}$ (upper row) and real-space $\Pi^{\alpha\beta}_{i-j}$ (lower row). From left to right we show $\Pi^{00}$, $\Pi^{z0}$, $\Pi^{zz}$ for parameters $t_{pp} = 1.0$, $T = 0.1$, $n_p = 0.1$. While $\Pi^{\alpha\beta}_{\boldsymbol{q}}$ are only $C_2$-symmetric, the resulting expression in the action is fully $C_4$-symmetric due to multiplication with the lattice functions $h_m, h_\eta$. We observe that $\Pi^{zz}_{\boldsymbol{q}}$ peaks at a non-zero wavevector showing that the maximal nematic response occurs at a finite $\boldsymbol{q}$.

Here, $\xi_\pm = \pm\epsilon_{\boldsymbol{q}} - \mu$ describes the two oxygen bands. Neglecting the interaction with the Néel magnetic background of the localized Cu spins, we obtain the oxygen bandstructure from the lattice function $h_{\boldsymbol{q}} = 1 - e^{iq_x} - e^{-iq_y} + e^{i(q_x-q_y)}$:

$$\epsilon_{\boldsymbol{q}} = t_{pp}|h_{\boldsymbol{q}}| = 4t_{pp}\Big|\sin\frac{q_x}{2}\Big|\Big|\sin\frac{q_y}{2}\Big|\,. \tag{S.31}$$

It is useful to introduce the density of states

$$g(\epsilon) = \frac{8}{(2\pi)^2}\int_{\cos^{-1}(1-\tilde{\mu})}^{\pi} dq_x \frac{\|\dot{\boldsymbol{\alpha}}(q_x)\|}{\|\nabla\xi_{\boldsymbol{q}=\boldsymbol{\alpha}(q_x)}\|} = \frac{8}{(2\pi)^2}\frac{4i}{\tilde{\mu}}\left[K\Big(\frac{4}{\tilde{\mu}^2}\Big) - F\Big(\frac{1}{2}\cos^{-1}(1-\tilde{\mu}), \frac{4}{\tilde{\mu}^2}\Big)\right], \tag{S.32}$$

where $\tilde{\mu} = \mu/(2t_{pp})$, $\boldsymbol{\alpha}(q_x) = \big(q_x, q_y(q_x)\big)$ with $q_y(q_x) = \cos^{-1}\Big(\frac{1-\tilde{\mu}^2-\cos q_x}{1-\cos q_x}\Big)$. The function $F(x)$ $[K(x)]$ is the [complete] elliptic integral of the first kind. We note that the density of states logarithmically diverges as $\epsilon \to 0$ due to a van-Hove singularity. We can now analyze the low and high-temperature behavior of the nematic response

$$\Pi^{zz}_{\boldsymbol{k}\to 0,\omega=0} = \frac{1}{t_{pp}}\int_0^2 d\epsilon\, \frac{g(\epsilon)}{\epsilon}\frac{\sinh\frac{\epsilon}{T}}{\cosh\frac{\epsilon}{T} + \cosh\frac{\mu}{T}} = \begin{cases} \frac{g(T)(2-|\mu|)}{t_{pp}} + \frac{e^{-|\mu|/T}|\log T|}{t_{pp}}\,, & \text{at low } T \ll 2t_{pp} \\ \frac{1}{2Tt_{pp}}\,, & \text{at high } T \gg 2t_{pp}\,, \end{cases} \tag{S.33}$$

where $2 - |\mu| \propto n_p$. At low temperatures, the response is dominated by the constant term proportional to $n_p$. As shown in Fig. 3 of the main text, the biquadratic exchange thus behaves in the experimentally relevant regime at low $T \ll 2t_{pp}$ as

$$\frac{K_0}{J} \propto \frac{J'^2}{J}\frac{n_p}{t_{pp}}\,. \tag{S.34}$$

### S1.D. Renormalization of biquadratic exchange coupling $K$ by quadrupolar oxygen density fluctuations

We now show that quadrupolar oxygen density fluctuations further enhance the biquadratic spin exchange from its bare value $K_0$ to a renormalized value $K > K_0$. These oxygen density fluctuations become stronger for increasing oxygen-oxygen repulsion $V_{pp}$. They are described by the bosonic Hubbard-Stratonovich fields $\Phi_q = (\psi_q, \phi_q)$ defined above Eq. (S.12). In the parameter regime we consider these fluctuations are non-critical and thus remain massive. Nematic order does not develop spontaneously, but occurs only in the presence of a conjugate symmetry-breaking field such as strain or as provided by the CuO chains in YBCO. After integration over the fermionic fields $p^\dagger_{qu\sigma}$ and $p_{qu\sigma}$ the action reads (see Eq. (S.22))

$$S = \int_q \sum_{\alpha,\beta} \big(\Phi^\dagger_{\boldsymbol{q}}\big)_\alpha \big(U_{\boldsymbol{q}}\big)_{\alpha\beta} \big(\Phi_{\boldsymbol{q}}\big)_\beta - \frac{1}{2} \int_q \Pi_q^{\alpha\beta} \Big[ \big(\Phi^*_q\big)_\alpha - \int_k \mathcal{S}_{k,-q} h_\alpha(\boldsymbol{k},\boldsymbol{q}) \Big] \Big[ \big(\Phi_q\big)_\beta - \int_k \mathcal{S}_{k,q} h_\beta(\boldsymbol{k},-\boldsymbol{q}) \Big] , \tag{S.35}$$

where $\alpha,\beta \in \{0,z\}$ and we identify $h_0(\boldsymbol{k},\boldsymbol{q}) \equiv h_m(\boldsymbol{k},\boldsymbol{q})$ and $h_z(\boldsymbol{k},\boldsymbol{q}) \equiv h_\eta(\boldsymbol{k},\boldsymbol{q})$. Performing the Gaussian integration over $\Phi^\dagger_{\boldsymbol{q}}$ yields

$$S = S_2^{\mathcal{S}^2} - \frac{1}{4} \sum_{\alpha,\beta,\gamma,\gamma'} \int_{q,k_1,k_2} \mathcal{S}_{k_1,q}\mathcal{S}_{k_2,q} h_\gamma(\boldsymbol{k}_1,-\boldsymbol{q}) h_{\gamma'}(\boldsymbol{k}_2,\boldsymbol{q}) (\tilde{U}_q^{-1})_{\alpha\beta} \Pi_q^{\gamma\alpha} \Pi_q^{\gamma'\beta} , \tag{S.36}$$

where we have defined

$$\big(\tilde{U}_q\big)_{\alpha\beta} = \big(U_{\boldsymbol{q}}\big)_{\alpha\beta} - \frac{1}{2}\Pi_q^{\alpha\beta} \tag{S.37}$$

with $U_{\boldsymbol{q}}$ given in Eq. (S.11). We note that the action in Eq. (S.36) is fully $C_4$ symmetric after summation over $\alpha,\beta,\gamma,\gamma'$, which we have explicitly verified. We can readily extract the renormalized response functions $\tilde{\Pi}^{\alpha\beta}_{\boldsymbol{q}}$ as

$$\tilde{\Pi}^{\gamma\gamma'}_{\boldsymbol{q}} = \Pi^{\gamma\gamma'}_{\boldsymbol{q}} + \frac{1}{2} \sum_{\alpha,\beta} \big(\tilde{U}^{-1}_{\boldsymbol{q}}\big)_{\alpha\beta} \Pi^{\gamma\alpha}_{\boldsymbol{q}} \Pi^{\gamma'\beta}_{\boldsymbol{q}} . \tag{S.38}$$

The renormalized biquadratic exchange interaction is therefore determined by the $zz$ component $\tilde{\Pi}^{zz}_{\boldsymbol{q}} = \Pi^{zz}_{\boldsymbol{q}} + \frac{1}{2}\sum_{\alpha,\beta}\big(\tilde{U}^{-1}_{\boldsymbol{q}}\big)_{\alpha\beta}\Pi^{z\alpha}_{\boldsymbol{q}}\Pi^{z\beta}_{\boldsymbol{q}}$. To gain more insight, we approximate the local response $\tilde{\Pi}^{zz}_{ii}$, which determines the biquadratic coupling $K = \frac{J'^2}{2}\tilde{\Pi}^{zz}_{ii}$ (see Eq. (S.29)), by the $\boldsymbol{q}=0$ component $\tilde{\Pi}^{zz}_{\boldsymbol{q}=0}$. Using that $(\tilde{U}^{-1}_{\boldsymbol{q}=0})_{11} = \frac{1}{U_{11} - \frac{1}{2}\Pi^{zz}_{\boldsymbol{q}=0}}$ with $U_{11}(\boldsymbol{q}=0) = \frac{1}{2}\frac{1}{V_{pp} - \frac{U_{pp}}{8}}$, the biquadratic exchange $K$, renormalized by quadrupolar oxygen density fluctuations, is given by

$$K = \frac{K_0}{1 - (V_{pp} - \frac{U_{pp}}{8})\Pi^{zz}_{ii}} . \tag{S.39}$$

We show $K/J$ as a function of hole doping $n_p$ in Fig. 2(a) of the main text for realistic parameters of the cuprates. The main insight from this result is that while on-site oxygen interactions $U_{pp}$ tend to reduce the biquadratic exchange, repulsive oxygen-oxygen interactions $V_{pp}$ enhance the biquadratic spin coupling $K > K_0$. For realistic parameters of the cuprates it holds that $V_{pp} \gg U_{pp}/8$ and the enhancement due to $V_{pp}$ is the dominant effect.

## S2. Nematic susceptibility within a soft-spin description of the half-filled $t-J-K$-model

In order to obtain an analytic understanding of the nematic response in the presence of a biquadratic exchange term $\propto K$ close to a Néel ordered state, we investigate a soft-spin version of the two-dimensional $t$-$J$-$K$-model at half-filling. We have also analyzed the nematic susceptibility in spatial dimensions $2 < d \leq 3$ and found that the results for the nematic response from $d=2$ remain qualitatively unchanged. After decoupling the biquadratic term at the expense of introducing the Hubbard-Stratonovich field $\varphi_r$, the action reads

$$S = \gamma \int_q \Big[ r_0 + q^2 + (\varphi_r + h_\varphi)(q_x^2 - q_y^2) + \gamma|\omega_n|^{2/z} \Big] M^\alpha_q M^\alpha_{-q} + \frac{\gamma^3 \tilde{u}}{2N} \int_{q_1,q_2,q_3} M^\alpha_{q_1} M^\alpha_{q_2} M^\beta_{q_3} M^\beta_{-q_1-q_2-q_3} + \int_r \frac{N\varphi_r^2}{2g} . \tag{S.40}$$

Here, $\boldsymbol{M}_q = (M_q^1, M_q^2, \dots, M_q^N)$ with $q = (i\omega_n, \boldsymbol{q})$ combining Matsubara frequency $i\omega_n = 2\pi i n T$ and momentum $\boldsymbol{q} = (q_x, q_y)$ denotes the (dimensionless) $N$-component staggered Néel magnetization. The integrations run over $\int_q = T\sum_{\omega_n}^{\Lambda_\omega}\int^{\Lambda}\frac{d^2q}{(2\pi)^2}$ with dimensionless momentum and frequency cutoffs $\Lambda$ and $\gamma\Lambda_\omega$ and $\int_r = \int_0^\beta d\tau \int d^2r$. The coupling constant $g \propto K/J$ is proportional to the ratio of biquadratic exchange $K$ to nearest-neighbor Heisenberg exchange $J$ in the spin model. The (bare) mass parameter $r_0$ controls the distance to the quantum critical point between Néel ordered and a paramagnetic $T = 0$ phases, and $\tilde{u} = u/\gamma$ is a dimensionless interaction constant. We have rescaled the interaction term $u/N$ to obtain a well-defined large-$N$ limit. In the following we set the dynamic critical exponent to $z = 2$, which describes damping due to particle-hole excitations in the presence of doped holes. We have added a source field $h_\varphi$ (denoted $h_r \equiv h_\varphi$ in the main text) that couples to homogeneous nematic order $\int_x h_\varphi \boldsymbol{M}_r(\boldsymbol{M}_{r+\hat{x}} + \boldsymbol{M}_{r-\hat{x}} - \boldsymbol{M}_{r+\hat{y}} - \boldsymbol{M}_{r-\hat{y}})$ with $\hat{x} = a_0(1,0)$ and $\hat{y} = a_0(0,1)$ with Cu-Cu distance $a_0$.

### S2.A. Nematic susceptibility $\chi_{\mathrm{nem},0}(r,T)$

The nematic susceptibility $\chi_{\mathrm{nem}}(T) = \int_0^{1/T} d\tau \sum_i \langle \mathcal{T}_\tau \varphi_i(\tau)\varphi_0(0)\rangle$ in Eq. (5) of the main text is obtained from the partition function $Z = \int \mathcal{D}(\boldsymbol{M}_q, \varphi_r) e^{-S}$ as

$$\chi_{\mathrm{nem}} = \frac{1}{\beta L^2}\frac{\partial^2 \ln Z}{\partial h_\varphi^2}\Big|_{h_\varphi=0} = \frac{\chi_{\mathrm{nem},0}}{1 - \frac{g}{N}\chi_{\mathrm{nem},0}} \tag{S.41}$$

with inverse temperature $\beta = 1/T$ and bare nematic susceptibility

$$\chi_{\mathrm{nem},0} = \frac{N}{g} - \frac{1}{\beta L^2 \langle \bar{\varphi}_r^2\rangle}\,. \tag{S.42}$$

To obtain this expression, we have shifted the field $\bar{\varphi}_r = \varphi_r + h_\varphi$ in Eq. (S.40) before taking the derivatives with respect to $h_\varphi$ and assumed the absence of an external field $h_\varphi = 0$ so that $\langle\bar{\varphi}_r\rangle^2 = 0$. We focus on static and homogeneous Hubbard-Stratonovich fields $\varphi_r$ and $\bar{\varphi}_r$, *i.e.*, both fields are independent of $r$. To analytically calculate the expectation value $\langle\bar{\varphi}_r^2\rangle$, we decouple the quartic term $\propto u$ in Eq. (S.40) by defining the (dimensionless) density $\rho_\psi = \frac{1}{N}\boldsymbol{M}_{\boldsymbol{x}}\cdot\boldsymbol{M}_{\boldsymbol{x}}$ and introducing a factor of unity as $1 = \int \mathcal{D}(\rho_\psi,\psi) e^{-\frac{1}{\gamma}\int_r (\boldsymbol{M}_x^2 - N\rho_\psi)\psi}$ [4], to arrive at

$$S = \gamma\int_q \left[r_0 + \psi + \boldsymbol{q}^2 + \bar{\varphi}_r(q_x^2 - q_y^2) + \gamma|\omega_n|\right]\boldsymbol{M}_{\boldsymbol{q}}\cdot\boldsymbol{M}_{-\boldsymbol{q}} + \frac{N}{\gamma}\int_r \frac{(\bar{\varphi}_r - h_\varphi)^2}{2\tilde{g}} + \frac{N}{\gamma}\int_r\Big(\frac{\tilde{u}}{2}\rho_\psi^2 - \psi\rho_\psi\Big)\,. \tag{S.43}$$

Here, the dimensionless field $\psi$ describes the renormalization of the mass from $r_0 \to r \equiv r_0 + \psi$. Separating longitudinal and transverse components $\boldsymbol{M}_r = (\sqrt{N}M, \boldsymbol{\pi}_r)$, where we restrict to homogeneous magnetic order $M$, and integrating over the $(N-1)$ transverse components, we arrive at the action density $s$:

$$s \equiv \frac{S}{\beta L^2\gamma^{-1}} = N(r_0+\psi)M^2 + \frac{N-1}{2}\gamma\int_q \ln\Big(r_0+\psi+\boldsymbol{q}^2+\bar{\varphi}_r(q_x^2-q_y^2)+\gamma|\omega_n|\Big) + \frac{N(\bar{\varphi}_r - h_\varphi)^2}{2\tilde{g}} + N\Big(\frac{\tilde{u}}{2}\rho_\psi^2 - \psi\rho_\psi\Big)\,. \tag{S.44}$$

Next, we expand the logarithm in small $\bar{\varphi}$ to find

$$\frac{s}{N} = \frac{\gamma}{2}\int_q \log r_q + \frac{\bar{\varphi}_r^2}{2}\Big(\frac{1}{\tilde{g}} - \gamma\int_q \frac{q^4\cos^2(2\theta)}{2r_q^2}\Big) + \frac{\tilde{u}}{2}\rho_\psi^2 - \psi\rho_\psi + \mathcal{O}(\bar{\varphi}^3)\,, \tag{S.45}$$

where $\boldsymbol{q} = |\boldsymbol{q}|(\cos\theta, \sin\theta)$ and $r_q = r + q^2 + \gamma|\omega_n|$ with $r = r_0 + \psi$. The generating functional of $\bar{\varphi}_r$ then reads

$$W[h_{\bar{\varphi}}] = \frac{1}{Z}\int \mathcal{D}(\bar{\varphi}_r) e^{-S - \bar{\varphi}_r h_{\bar{\varphi}}} = \exp\left[\frac{h_{\bar{\varphi}}^2}{2N}\frac{\gamma}{\beta L^2}\Big(\frac{1}{\tilde{g}} - \gamma\int_q \frac{q^4\cos^2(2\theta)}{2r_q^2}\Big)^{-1}\right] \tag{S.46}$$

and the bare nematic susceptibility $\chi_{\mathrm{nem},0}$ in Eq. (S.42) follows to

$$\chi_{\mathrm{nem},0} = \frac{N}{2}T\sum_{\omega_n}\int_0^\Lambda \frac{d^2q}{(2\pi)^2}\frac{q^4\cos^2(2\theta)}{(r + q^2 + \gamma|\omega_n|)^2} = \frac{N}{(2\pi)^2\gamma}\int_0^{\gamma\Lambda_\omega} d\omega \int_0^\Lambda dq \frac{\omega(r+q^2)q^5}{[(r+q^2)^2+\omega^2]^2}\coth\Big(\frac{\omega}{2\gamma T}\Big)\,. \tag{S.47}$$

In the final step we have gone from summation over Matsubara frequencies to integration along the real frequency axis, and performed the angular integration over $\theta$. Note that while $\omega_n$ has units of energy, the integration variable

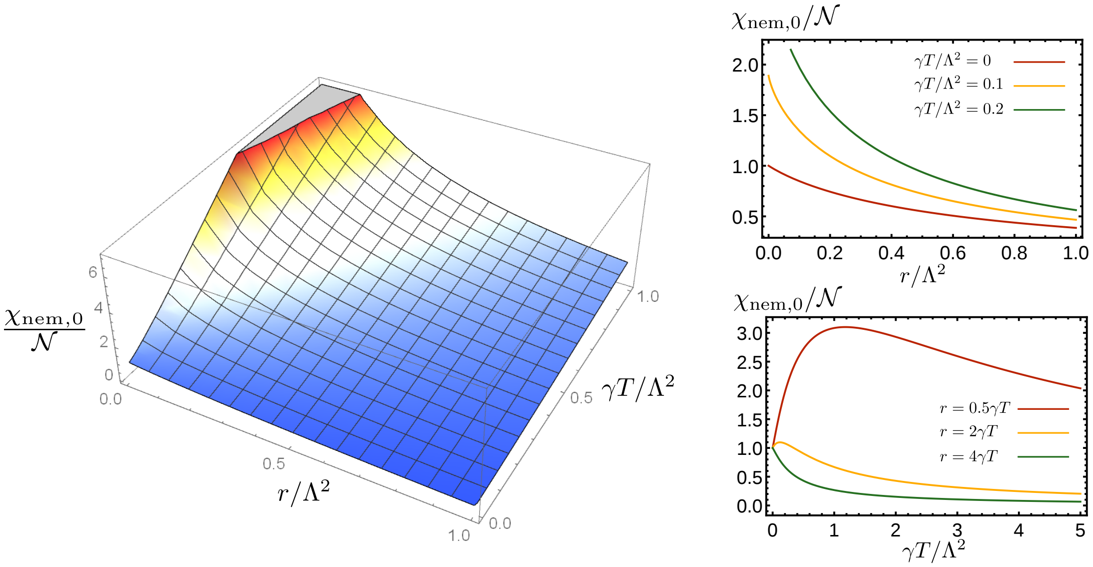


FIG. S.2. (Left) Nematic susceptibility $\chi_{nem,0}/\mathcal{N}$ with cutoff dependent normalization factor $\mathcal{N} = N\Lambda^4/(64\pi^2\gamma)$ as a function of $\tilde{r} = r/\Lambda^2$ and $\tilde{T} = \gamma T/\Lambda^2$. We observe that for fixed temperature $T$, the susceptibility increases as $r \propto \xi^{-2}$ decreases (see panel on the upper right). This shows that Néel fluctuations enhance the nematic susceptibility. As a function of temperature, we observe that $\chi_{nem,0}/\mathcal{N}$ starts out from a non-zero value at $T = 0$ that is equal to $\chi_{nem,0}(r = 0, T = 0)/\mathcal{N} = 1$ at the quantum critical point and smaller for $r > 0$. The finite-temperature behavior of $\chi_{nem,0}[r(T), T]/\mathcal{N}$ depends on microscopic details as expected for a non-universal quantity. The panel on the lower right shows the finite-$T$ behavior above the quantum critical point for different values of the slope $r(T) = a\gamma T$, $a = \{0.5, 2, 4\}$. For $a < \pi$ ($a > \pi$) the susceptibility first increases (decreases) linearly as a function of $T$, at larger $T$ it decays to zero. It reaches a maximum when $\tilde{r} \approx 1$, which marks the transition into the lattice high-$T$ regime.

$\omega$ is dimensionless by expressing energies in units of $\gamma^{-1}$. While we must keep both momentum and frequency cutoff $\Lambda$ and $\gamma\Lambda_\omega$ finite when we solve for $r(r_0, T)$ in the following section (using the large-$N$ approximation), we may take the limit $\gamma\Lambda_\omega \to \infty$ in Eq. (S.47). This allows us to exactly perform the momentum and frequency integrations and completely absorb the cutoff $\Lambda$ by expressing $\chi_{nem,0}$ in terms of the (dimensionless) variables $\tilde{r} = r/\Lambda^2$ and $\tilde{T} = \gamma T/\Lambda^2$ as

$$\chi_{nem,0} = \frac{N\Lambda^4}{64\pi^2\gamma}\Bigg[4\pi\tilde{T}\Big[\frac{2\tilde{r}+1}{\tilde{r}+1} + 2\tilde{r}\log\frac{\tilde{r}}{\tilde{r}+1}\Big] + 2\psi\Big(1+\frac{\tilde{r}+1}{2\pi\tilde{T}}\Big)$$
$$- 8\pi\tilde{T}\Big\{\log\Gamma\Big(\frac{\tilde{r}+1+2\pi\tilde{T}}{2\pi\tilde{T}}\Big) + 2\pi\tilde{T}\Big[\psi^{(-2)}\Big(1+\frac{\tilde{r}}{2\pi\tilde{T}}\Big) - \psi^{(-2)}\Big(1+\frac{r+1}{2\pi\tilde{T}}\Big)\Big]\Big\}\Bigg]. \quad (S.48)$$

In Fig. S.2, we show $\chi_{nem,0}/\mathcal{N}$, where $\mathcal{N} = N\Lambda^4/(64\pi^2\gamma)$ as a function of $\tilde{r} = r/\Lambda^2$ and $\tilde{T} = T/\Lambda^2$. Note that $\mathcal{N} \equiv \chi_{nem,0}(r = 0, T = 0)$ is the value of the susceptibility at the quantum critical point. Along a path of constant temperature, the nematic susceptibility increases as $r$ decreases, which is also shown in the upper right panel of Fig. S.2. Decreasing $r \propto \xi^{-2}$ implies an increasing magnetic Néel correlation length as one approaches the $T = 0$ quantum critical point or the renormalized classical regime with exponentially large magnetic correlation length at $T > 0$. The nematic susceptibility thus increases as a result of larger magnetic Néel fluctuations. Our analysis also reveals that while for classical spins $\chi_{nem,0}$ vanishes as $T \to 0$, quantum fluctuations render the zero temperature limit of $\chi_{nem,0}$ finite.

To plot $\chi_{nem,0}$ along a path of constant $r_0$, which controls the distance to the quantum critical point beyond which Néel order disappears, one needs to solve for the renormalized mass parameter $r(T, r_0)$. At finite temperatures above the quantum critical point, one finds $r(T, r_{0,c}) = a\gamma T \propto T$ with a non-universal proportionality constant $a$ that depends on microscopic details of the system. As shown in the lower right panel of Fig. S.2, the shape of $\chi_{nem,0}$ crucially depends on the value of the slope parameter $a$, which controls the relative importance of quantum and thermal fluctuations. For small values of $a < \pi$, $\chi_{nem,0}$ develops a pronounced finite-temperature peak, whose amplitude increases with decreasing $a$. This behavior of $\chi_{nem,0}$ closely resembles the behavior found within the classical Monte-Carlo simulations (see Fig. 2 of the main text), and show that thermal fluctuations are dominant for $a < \pi$. In contrast, for larger values $a > \pi$, $\chi_{nem,0}$ peaks at $T = 0$ and is a monotonically decreasing function for

finite $T$, showing the dominance of quantum fluctuations in this case.

### S2.B. Large-$N$ analysis of the nematic susceptibility

In order to determine the effective mass parameter $r(T, \delta r_0)$ as a function of temperature $T$ and distance to the quantum critical point $\delta r_0 = r_0 - r_{0,c}$, we consider the limit of large-$N$, where the partition function is governed by the saddle point of the action in Eq. (S.40). Finding the saddle-point of the action in Eq. (S.44) in the absence of nematic order, leads to the well-known large-$N$ self-consistency equations [4, 5]: $rM = 0$ with $r = r_0 + \psi$; $\rho_\psi = \gamma\psi/u$ and

$$r = r_0 + uM^2 + \frac{u}{2}\int_q \frac{1}{r + q^2 + \gamma|\omega_n|} \tag{S.49}$$

The equation requires a finite frequency cutoff $\Lambda_\omega$. For the results of $\chi_{\text{nem},0}$ in Fig. 2 of the main text, we have therefore numerically solved these equations for finite momentum $\Lambda$ and (dimensionless) frequency cutoffs $\gamma\Lambda_\omega$, which yields $r(r_0, T)$ shown in Fig. S.3. The qualitative behavior of $\chi_{\text{nem},0}$ as discussed in the previous section does not depend on the exact value of $\gamma\Lambda_\omega$ and $\Lambda$ as long as both cutoffs are much larger than $r, \gamma T \ll \Lambda, \gamma\Lambda$.

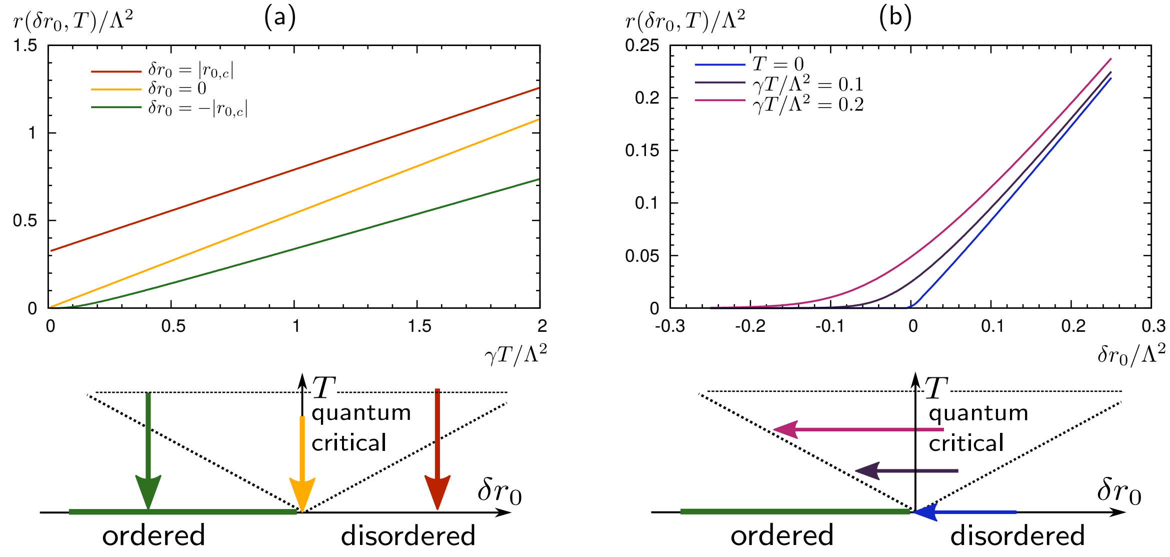


FIG. S.3. Large-$N$ solutions for the "mass" parameter $r(r_0, T) \propto \xi^{-2}$, where $\xi$ is the magnetic correlation length for Néel order. This parameter controls the distance to criticality. The resulting nematic susceptibilities are shown in Fig. 3 of the main text. Panels (a) and (b) correspond to same panels in Fig. 3 of the main text. The left panel (a) shows $r$ as a function of temperature at fixed distance to criticality $\delta r_0$, as depicted in the schematic diagram with vertical paths corresponding to different values of $\delta r_0$. For $\delta r_0 > 0$ (red), $r$ approaches a finite value as $T \to 0$ corresponding to a finite magnetic correlation length in the quantum disordered phase. In contrast, for $\delta r_0 \leq 0$ (yellow, green), $r \to 0$ as $T \to 0$. Approaching the quantum critical point (yellow), one finds $r = a\gamma T$ with non-universal slope $a$ that depends among others on the size of the interactions $u/\gamma$. Larger $u/\gamma$ yields a larger $a$. Approaching the magnetically ordered phase (green), we observe a change in functional behavior of $r(T)$ as we cross from the quantum critical to the renormalized classical regime. In the quantum critical regime at higher $T$, one finds $r(T) \propto T$. In contrast, in the renormalized classical regime at lower $T$, it holds $r(T) \propto T\exp(-\Delta(\delta r_0)/T)$, where $\Delta$ depends on the spin stiffness in the ordered phase (rigidity towards magnetic fluctuations) [5]. The right panel (b) corresponds to changing $\delta r_0$ at fixed temperature $T$. In an experiment, this corresponds, for example, to tuning the chemical composition or pressure. Importantly, we observe that $r \propto \xi^{-2}$ is a monotonously decreasing function for decreasing $\delta r_0$, *i.e.*, approaching the quantum critical point or the renormalized classical region. While in two dimensions the Hohenberg-Mermin-Wagner theorem ensures a finite correlation length $r > 0$ at any finite temperature $T$, one finds that $r(T)$ becomes exponentially small, because $\xi$ becomes exponentially large, in the renormalized classical regime to the left of the dashed line. From Fig. 2 of the main text, we conclude that the nematic susceptibility $\chi_{\text{nem}}$ increases if $r$ decreases or $\xi$ increases, which shows that larger Néel fluctuations enhance the nematic response.

### S3. Spin-wave treatment of $t - J - K$ model at half-filling

At half-filling the Hamiltonian in Eq. (1) of the main text describes localized Cu spins interacting via nearest-neighbor Heisenberg exchange interaction $J$ and a biquadratic exchange interaction $K$. Additional weaker next-nearest neighboring and ring-exchange terms may be added to obtain agreement with the experimental spin-wave spectra [6]. Since these terms do not change our conclusions, we do not explicitly consider them below. Note that we include a realistic ferromagnetic exchange coupling $J_2 = -0.1J$ in our Monte-Carlo simulations (see Fig. 2 of the main text).

We now show that the biquadratic spin exchange term $\propto K$ does not modify the spin-wave spectrum. Adding such a term in the Hamiltonian is thus fully consistent with previous experimental results of the spin-wave spectrum. We derive our results starting from the $J$-$K$ model spin Hamiltonian in Eq. (1) of the main text

$$H = \frac{J}{2}\sum_{i=1}^{N_L}\sum_{\delta_\nu=\delta_1}^{\delta_4} \boldsymbol{S}_i \boldsymbol{S}_{i+\delta_\nu} - \frac{K}{4S^2}\sum_{i=1}^{N_L}\Big[\boldsymbol{S}_i\Big(\boldsymbol{S}_{i+\hat{x}} + \boldsymbol{S}_{i-\hat{x}} - \boldsymbol{S}_{i+\hat{y}} - \boldsymbol{S}_{i-\hat{y}}\Big)\Big]^2 . \tag{S.50}$$

Here, $\{\delta_\nu\} = \{\pm\hat{x}, \pm\hat{y}\}$ connect nearest-neighbors Cu sites. Let us calculate the spin-wave spectrum around the Néel state. As this corresponds to a large-$S$ limit, we have rescaled the biquadratic term. We follow the standard procedure of Holstein-Primakoff spin-wave calculations [7] and begin with defining local triads $\boldsymbol{n}_{1,\boldsymbol{R}_i} = \big(\cos(\boldsymbol{Q}\cdot\boldsymbol{R}_i), 0, -\sin(\boldsymbol{Q}\cdot\boldsymbol{R}_i)\big)$, $\boldsymbol{n}_2 = \big(0,1,0\big)$ and $\boldsymbol{n}_{3,\boldsymbol{R}_i} = \big(\sin(\boldsymbol{Q}\cdot\boldsymbol{R}_i), 0, \cos(\boldsymbol{Q}\cdot\boldsymbol{R}_i)\big)$ with Néel ordering wavevector $\boldsymbol{Q} = (\pi,\pi)$. Expressing the spins in terms of this local coordinate system $\boldsymbol{S}_i = \sum_\alpha \tilde{S}_i^\alpha \boldsymbol{n}_{\alpha,\boldsymbol{R}_i}$, the Hamiltonian takes the form (suppressing the tilde)

$$H = \frac{J}{2}\sum_{i,\delta_\nu,\alpha,\beta} S_i^\alpha S_{i+\delta_\nu}^\beta n_{\beta,\delta_\nu}^\alpha + \frac{K}{4S^2}\sum_i\sum_{\alpha,\beta}\Big[n_{\beta,\delta_\nu}^\alpha S_i^\alpha\Big(S_{i+\hat{x}}^\beta + S_{i-\hat{x}}^\beta - S_{i+\hat{y}}^\beta - S_{i-\hat{y}}^\beta\Big)\Big]^2 \tag{S.51}$$

with $n_{\beta,\delta_\nu}^\alpha = \delta_{\alpha\beta}(-\delta_{x\alpha} + \delta_{y\alpha} - \delta_{z\alpha})$. A transformation to momentum space via $\boldsymbol{S}_i = \frac{1}{\sqrt{N_L}}\sum_{\boldsymbol{p}\in BZ} e^{i\boldsymbol{p}\cdot\boldsymbol{R}_i}\boldsymbol{S}_{\boldsymbol{p}}$ yields

$$H = 2J\sum_{\boldsymbol{p}}\sum_\alpha f_{\boldsymbol{p}} S_{\boldsymbol{p}}^\alpha S_{-\boldsymbol{p}}^\alpha n_{\alpha,\delta_\nu}^\alpha + \frac{K}{N_L S^2}\sum_{\boldsymbol{p},\boldsymbol{q},\boldsymbol{k}}\sum_{\alpha,\beta} S_{\boldsymbol{p}+\boldsymbol{k}}^\alpha S_{-\boldsymbol{p}}^\alpha S_{\boldsymbol{q}-\boldsymbol{k}}^\beta S_{-\boldsymbol{q}}^\beta n_{\alpha,\delta_\nu}^\alpha n_{\beta,\delta_\nu}^\beta (\cos p_x - \cos p_y)(\cos q_x - \cos q_y)\,, \tag{S.52}$$

where we have defined the lattice function $f_{\boldsymbol{p}} = \frac{1}{4}\sum_{\delta_\nu} e^{-i\boldsymbol{p}\delta_\nu} = \frac{1}{2}(\cos p_x + \cos p_y)$. To obtain the spin-wave spectrum, we now express spin operators in terms of Holstein-Primakoff bosons $S_{\boldsymbol{q}}^x = \sqrt{\frac{S}{2}}\Big(b_{-\boldsymbol{q}}^\dagger + b_{\boldsymbol{q}}\Big)$, $S_{\boldsymbol{q}}^y = i\sqrt{\frac{S}{2}}\Big(b_{-\boldsymbol{q}}^\dagger - b_{\boldsymbol{q}}\Big)$ and $S_{\boldsymbol{q}}^z = \sqrt{N_L}S\delta_{\boldsymbol{q},0} - \frac{1}{\sqrt{N_L}}\sum_{\boldsymbol{k}} b_{\boldsymbol{k}-\boldsymbol{q}}^\dagger b_{\boldsymbol{k}}$. The classical ground state energy follows as the $\mathcal{O}(S^2)$-term to $H^{(S^2)}/(N_L S^2) = -2J$. Note that the energy of the biquadratic term vanishes in the Néel state.

The next lowest order in $S$ is quadratic in the bosons and yields upon diagonalization the spin-wave spectrum. Keeping the quadratic terms, yields

$$H_J^{(S)} = 2JS\sum_{\boldsymbol{q}}\Big(2b_{\boldsymbol{q}}^\dagger b_{\boldsymbol{q}} - f_{\boldsymbol{q}}(b_{-\boldsymbol{q}}^\dagger b_{\boldsymbol{q}}^\dagger + b_{\boldsymbol{q}}b_{-\boldsymbol{q}})\Big) \tag{S.53}$$

$$H_K^{(S)} = 0\,, \tag{S.54}$$

Most importantly, according to Eq. (S.54), the biquadratic term does not contribute to the spin-wave spectrum at order $\mathcal{O}(S)$. Intuitively, the vanishing of the biquadratic contribution to the spin-wave spectrum follows from the observation that inserting the classical spin state into one of the factors $\boldsymbol{S}_i(\boldsymbol{S}_{i+\hat{x}} + \boldsymbol{S}_{i-\hat{x}} - \boldsymbol{S}_{i+\hat{y}} - \boldsymbol{S}_{i-\hat{y}})$ gives zero, because the term in the brackets vanishes in the Néel state. More explicit, this result can be seen already from Eq. (S.52): to obtain a term of $\mathcal{O}(S)$ the term in the bracket has to be of order $S^3$ in order to combine with the prefactor $K/S^2$ to a term of $\mathcal{O}(S)$. There are two possibilities, which both vanish: (i) $zzzz$ terms, *i.e.*, selecting 3 Kronecker symbols and selecting one term of the form $\sum_{\boldsymbol{k}} b_{\boldsymbol{k}-\boldsymbol{q}}^\dagger b_{\boldsymbol{k}}$ (from $S_{\boldsymbol{q}}^z$). The Kronecker symbols enforce $\boldsymbol{p} = \boldsymbol{q} = \boldsymbol{k} = 0$ and therefore $\cos p_x - \cos p_y = 0$ and $\cos q_x - \cos q_y = 0$. The other possibility are (ii) terms of the form $(zzxx + zzyy + xxzz + yyzz)$, *i.e.*, selecting two Kronecker symbols and two $S^x$, $S^y$ terms. The Kronecker symbols give either $\boldsymbol{p} = \boldsymbol{k} = 0$ or $\boldsymbol{q} = \boldsymbol{k} = 0$ and thus one of the cos-terms vanishes: $\cos p_x - \cos p_y = 0$ or $\cos q_x - \cos q_y = 0$.

We finally want to note an interesting observation. If one uses the well-known relations for spin-1/2 operators $\big(\boldsymbol{S}_i\cdot\boldsymbol{S}_j\big)^2 = \frac{3}{16} - \frac{1}{2}\boldsymbol{S}_i\cdot\boldsymbol{S}_j$ and $\big(\boldsymbol{S}_i\cdot\boldsymbol{S}_j\big)\big(\boldsymbol{S}_i\cdot\boldsymbol{S}_k\big) = \frac{1}{4}\boldsymbol{S}_j\cdot\boldsymbol{S}_k + \frac{i}{2}\boldsymbol{S}_i\cdot(\boldsymbol{S}_j\times\boldsymbol{S}_k)$, one may rewrite the biquadratic term as a sum of three spin exchange terms such that the spin Hamiltonian in Eq. (S.50) takes the form

$$H = \frac{1}{2}(J + \frac{K}{4S^2})\sum_i\sum_\delta \boldsymbol{S}_i\cdot\boldsymbol{S}_{i+\delta} + \frac{K}{8S^2}\sum_i\sum_{\delta'} \boldsymbol{S}_i\cdot\boldsymbol{S}_{i+\delta'} - \frac{K}{16S^2}\sum_i\sum_{\delta''} \boldsymbol{S}_i\cdot\boldsymbol{S}_{i+\delta''}\,. \tag{S.55}$$

Interestingly, there now appears a non-zero contribution of the $K$-dependent exchange terms to the spin-wave spectrum. Note that this explicitly shows that using the above spin transformation rules valid for spin-1/2 does not commute with taking the large-$S$ limit to derive the spin-wave spectrum.

### S4. Details on the Monte-Carlo simulations

The Monte Carlo simulations were carried out at 100 equally spaced temperature points in the interval $0.001 < T/J < 2.971$. We applied a combination of single-move Metropolis Monte Carlo steps and non-local parallel-tempering-exchange steps between neighboring temperature configurations. The simulations shown in Fig. 2 of the main text were carried out for systems of $40 \times 40$ spins and biquadratic exchange couplings $K/J = \{0.0, 0, 35, 0.45\}$. We consider a ferromagnetic next-nearest-neighbor exchange coupling $J_2 = -0.1J$ as well. Note that the ground state phase transition in the classical model between Néel and collinear order occurs at $J/2 = J_2 + K$. Following thermalization, the averages were computed for each temperature with at least $4.5 \times 10^6$ Monte Carlo sweeps (MCS). The error bars were estimated by using the well-known Jackknife procedure.


[1] V. J. Emery, Phys. Rev. Lett. **58**, 2794 (1987).
[2] E. Kolley, W. Kolley, and R. Tiertz, J. Phys. C **4**, 3517 (1992).
[3] J. Zaanen and A. M. Oleś, Phys. Rev. B **37**, 9423 (1988).
[4] J. Zinn-Justin, *Quantum Field Theory and Critical Phenomena* (Oxford University Press, New York, NY, USA, 2002).
[5] S. Sachdev, *Quantum Phase Transitions* (Cambridge University Press, Cambridge, U.K., 1999).
[6] R. Coldea, S. M. Hayden, G. Aeppli, T. G. Perring, C. D. Frost, T. E. Mason, S.-W. Cheong, and Z. Fisk, Phys. Rev. Lett. **86**, 5377 (2001).
[7] A. Auerbach, *Interacting Electrons and Quantum Magnetism* (Springer-Verlag, New York, 1994).
